# Supplementary material for: DiscDiff: Latent Diffusion Model for DNA Sequence Generation
Source: arXiv:2402.06079 source file (2024-04-17)
Supplement: Supplementary file 1 [file metric-definition.tex]

\section{Metric Definition}

\paragraph{Motif Distribution correlation (MotifCor).)}
The Pearson correlation coefficient, denoted as \( r \), for two motif distributions \( X \) and \( Y \) is defined as:

\[
    r = \frac{\sum_{i=1}^{n} (x_i - \bar{x})(y_i - \bar{y})}{\sqrt{\sum_{i=1}^{n} (x_i - \bar{x})^2 \sum_{i=1}^{n} (y_i - \bar{y})^2}}
\]

where:
\begin{itemize}
    \item \( x_i \) and \( y_i \) are the individual observed values in distributions \( X \) and \( Y \), respectively.
    \item \( \bar{x} \) and \( \bar{y} \) are the means of distributions \( X \) and \( Y \).
    \item \( n \) is the number of paired observations.
\end{itemize}

This formula measures the degree of linear correlation between two datasets, ranging from -1 (indicating a perfect negative correlation) to +1 (indicating a perfect positive correlation), with 0 indicating no linear correlation.
